# Supplementary material for: Realistic Defocus Blur for Multiplane Computer-Generated Holography
Source: arXiv:2205.07030 source file (2023-02-06)
Supplement: Supplementary file 1 [file supplementary.pdf]

# Supplementary: Realistic Defocus Blur for Multiplane Computer-Generated Holography

KORAY KAVAKLI, Koç University, Turkey

YUTA ITOH, Tokyo Institute of Technology, Japan

HAKAN UREY, Koç University, Turkey

KAAN AKŞIT, University College London, UK

## Reference Format:

Koray Kavaklı, Yuta Itoh, Hakan Urey, and Kaan Akşit. 20XX. Supplementary: Realistic Defocus Blur for Multiplane Computer-Generated Holography. In . ACM, New York, NY, USA, 9 pages. <https://doi.org/XXXXXXX.XXXXXXX>

## 1 GAZE-CONTINGENT LOSS

Our proposed loss function,  $\mathcal{L}_m$ , can further be improved in the presence of a visual saliency or gaze location mask,  $S$ , leading to our salient loss function,  $\mathcal{L}_s$ , described as

$$\mathcal{L}_s = m_0 \mathcal{L}_2(SP_k, SI_k) + m_1 \mathcal{L}_2(SM_k P_k, SM_k I_k). \quad (1)$$

Note that  $\mathcal{L}_s$  is optional and only useful when a saliency map,  $S$ , is provided among with  $P_{target}$  and  $V_{depth}$ .

## 2 OPTICAL BEAM PROPAGATION

A phase-only hologram is described as a two-dimensional array filled with phase values and typically described with a complex notation as  $O_h = e^{j\phi(x,y)}$ , where  $\phi$  represents the phase delay introduced by each pixel at a phase-only hologram. Holographic displays typically represent holograms,  $O_h$  with programmable SLMs. Meanwhile, a coherent beam illuminating a phase-only hologram,  $U_i$ , is also described as a two-dimensional array. Note that  $U_i$  is an oscillating electric field described as  $U_i = A_0 e^{j(k\vec{r} + \phi_0(x,y))}$ , where  $A_0$  represents the amplitude of the optical beam,  $k$  represents the wavenumber that can be calculated as  $\frac{2\pi}{\lambda}$ ,  $\lambda$  represents the wavelength of light, and  $\phi_0$  represents the initial phase of the optical beam. In calculation,  $A_0$  is often considered  $A_0 = 1$  for an ideal collimated beam, while  $\phi_0$  is assumed to be a two-dimensional array filled with random values between zero to  $2\pi$ . Finally, leading to simplification of  $U_i$  as  $e^{j\phi_0}$ . In simple terms, as  $U_i$  illuminates  $O_h$ ,  $U_i$  by modulated with  $O_h$ , forming a new modulated beam  $U_m$  that is calculated as

$$U_m = U_i O_h = e^{j(\phi(x,y) + \phi_0(x,y))}. \quad (2)$$

A modulated beam,  $U_m$ , has to propagate in free-space from the hologram plane (SLM plane) towards a target depth plane to reconstruct images at various depth planes. Propagation of optical beams from one plane to another follows the theory and method introduced by Rayleigh-Sommerfeld diffraction integrals [4]. This diffraction integral's first solution, the Huygens-Fresnel principle, is expressed as follows:

$$u(x, y) = \frac{1}{j\lambda} \iint u_0(x, y) \frac{e^{jkr}}{r} \cos(\theta) dx dy, \quad (3)$$

---

arXiv

Supplementary, ,

© 20XX authors.

ACM ISBN 978-1-4503-XXXX-X/18/06...\$YY.YY

<https://doi.org/XXXXXXX.XXXXXXX>

where resultant field,  $U(x, y)$  is calculated by integrating over every point across hologram plane,  $U_0(x, y)$  represents the optical field in the hologram plane for every point across XY axes,  $r$  represents the optical path between a selected point in hologram plane and a selected point in target plane,  $\theta$  represents the angle between these points. The angular spectrum method, an approximation of the Huygens-Fresnel principle, is often simplified into a single convolution with a fixed spatially invariant complex kernel,  $h(x, y)$  [11],

$$u(x, y) = u_0(x, y) * h(x, y) = \mathcal{F}^{-1}(\mathcal{F}(u_0(x, y))\mathcal{F}(h(x, y))). \quad (4)$$

In our implementations, we rely on a fundamental library for optical sciences [1], which provides a differentiable version of various optical beam propagation methods. Therefore, our methods can work with other beam propagation approximations.

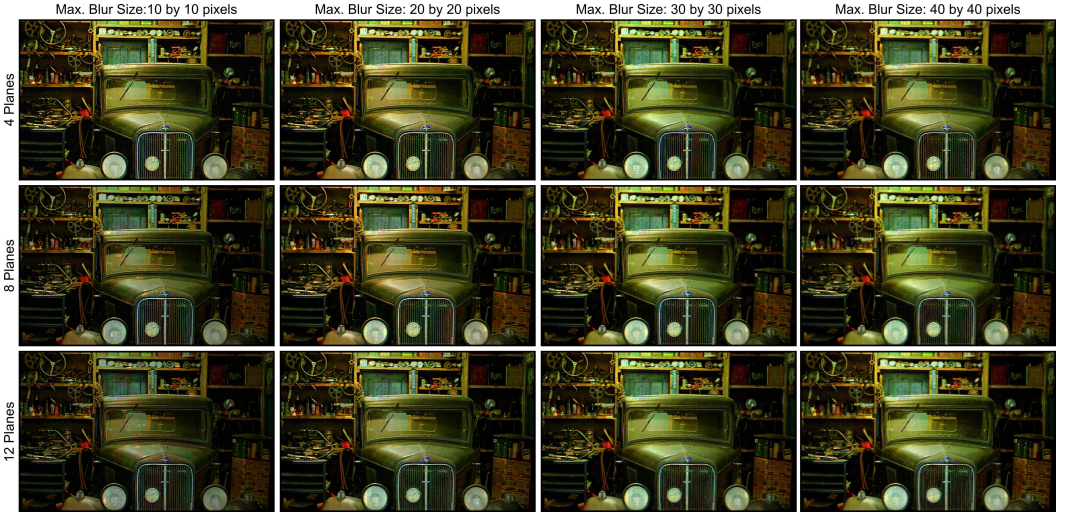

Fig. 1. The number of depth planes and blur size. We show actual captures from our holographic display with a 20 ms exposure time and fixed laser powers. At each row, we quantize our depth target into various numbers of planes (4-8-12 planes). In each column, we change the maximum blur kernel sizes. Our results suggest that our method supports various quantization levels of depth while providing tunable blur sizes, opening up the possibility to stylize images according to a viewer’s taste.

## ADDITIONAL RESULTS

In addition to the main manuscript, here, we provide additional results from our simulations and our holographic display, which we provide in Figure 2 and Figure 3. These results are captured when images are reconstructed on the SLM plane with a 1 mm distance between each plane. There is six target image plane in this case. In the future, we also plan on exploring learned models [5] for improving the visual quality further and mitigating imperfections in hardware setup.

### BLUR SIZE AND NUMBER OF DEPTH PLANES.

Our multiplane CGH generation pipeline can generate images with various multiple quantization levels in depth. In addition, our CGH pipeline offers control over blur size, rendering scenes in a styled way according to a viewer’s taste. In our method, Gaussian Kernels can be replaced with Zernike polynomials in the future to support the prescription of a viewer. Here, we provide the

evidence that our CGH pipeline can provide images with various quantizations and blur sizes as in Figure 1.

## DETAILS OF DISPLAY PROTOTYPE

This section describes our hardware implementation details of the holographic display prototype. The SLM in our system is Holoeye Pluto-VIS which contains a driver unit with a DVI connection and a phase-only LCoS microdisplay with full HD resolution ( $1920 \times 1080$  pixels),  $8 \mu\text{m}$  pixel pitch, and an active area of  $15.36 \times 8.64 \text{ mm}$  ( $0.7''$  Diagonal). It can address 8 Bit (256 grey levels) depth levels. Our laser source is LASOS MCS-4 laser module that is fiber-coupled to a single-mode fiber. An Arduino UNO is connected to the laser interface to modulate our laser source's RGB channels. The optical reconstructions at each plane are captured individually with the help of a linear stage mounted with the camera on top it. In Figure 4, we provide USAF 1951 and Indian Head Pattern charts to assess the quality of our holographic display prototype.

## AUGMENTED REALITY NEAR-EYE DISPLAY APPLICATION

Our work can also be used in Augmented Reality (AR) near-eye displays [6]. Here, we show a sample application note, where we modified our holographic display prototype to get to an AR application example. Our modification involves adding a standard mirror after the  $4f$  imaging system so that the optical path can be steered at  $110$  degrees. Along the steered optical path axis, we add a lens (Thorlabs LA11-45-A) and a beamsplitter to imitate an eyepiece of an AR near-eye display. Our camera, Nikon D5300 equipped with AF Nikkor 50mm  $f/1.8D$  follows the beam splitter. In Figure 5, we provide several photographs to demonstrate our configuration.

To evaluate our prototype, we have constructed an actual scene where we put real objects at the targeted virtual image distances. We provide our sample captures from this AR application in Figure 6. The real objects, Rubik's Cube, train, and snowman, are located at  $45 \text{ cm}$ ,  $65 \text{ cm}$ , and  $100 \text{ cm}$  with respect to the user's view.

## LONG PROJECTION DISTANCES

The edge fringe artifacts become more apparent when image planes are reconstructed further away from the SLM. In order to demonstrate this effect and validate our method for long projection distances, we built another holographic display prototype which forms the image planes at  $15 \text{ cm}$ ,  $14.5 \text{ cm}$  and  $14.0 \text{ cm}$  away from the SLM. Figure 7 provides a detailed overview of our optical schematic and photographs of this prototype. The optical path of this display prototype starts from a laser light source, LASOS MCS4, which combines three separate laser light sources. Thorlabs LA1708-A plano-convex lens with a  $200 \text{ mm}$  focal length collimates the light emitted from the single-mode fibre output. The linearly polarized collimated beam bounces off the beamsplitter, Thorlabs BP245B1, towards our phase-only SLM, Holoeye Pluto-VIS ( $1920 \times 1080 \text{ px}$ ,  $8 \mu\text{m}$ ). The phase-modulated beam from our phase-only SLM arrives at a combination of  $500 \text{ mm}$  and  $250 \text{ mm}$  focal length plano-convex/bi-convex lenses, Thorlabs LA1908-A & LB1056-A. A pinhole aperture, Thorlabs SM1D12, follows the lenses at a focal length away. We capture the image reconstructions with a lensless image sensor, Point Grey GS3-U3-23S6M-C USB 3.0, located on an X-stage (Thorlabs PT1/M travel range:  $0\text{-}25 \text{ mm}$ , precision:  $0.01 \text{ mm}$ ).

In Figure 8, we provide a comparison between naive SGD, tensor holography, and our method for long projection distances.

## DISCUSSION

Using our proof-of-concept holographic display, we demonstrated a complete multiplane CGH calculation pipeline with near-accurate defocus blur. While we noticeably mitigate edge fringe

issues and our results approximate natural focus blur, there are remaining issues and potential new research paths.

*Perceptual Holography.* Recent literature [12] [2, 3] promises to take advantage from the qualities of human visual system by introducing new loss functions that help reconstruct images at peripheral vision with perceptual guidance and gaze-contingency. Although these works open up a new combination in research, these works can be best described as first stabs at achieving true perceptual realism. Future perceptual graphics and computational displays research must find ways to carefully tune the image spatiotemporal qualities of holography to achieve life-like visuals.

*Occlusion in multiplanar holography.* A change in a user’s point-of-view when observing multi-plane images can lead to occlusion related issues with most multiplane CGH approaches, including ours. These occlusions manifest as missing image parts or images that look “holo” (seeing one object inside another). Hence, addressing the occlusion issue is essential and an outstanding scientific question in multiplane CGH. Further research in data representations in multiplane is also required to provide occlusions similar to point-based representations in the literature [9].

*Practical issues.* Despite the well-known advantages of CGHs, there are still many challenges to be addressed, including field-of-view [7], depth-of-field [8], and speckle noise [10]. Another challenge in working with a laser-based display system is dust and imperfections on optical components such as diamond turning marks, which causes diffraction problems and undesired fringe patterns on the holograms. We believe holographic displays need to support imperfect optical components to be practical and highly reproducible at the consumer level. These practical issues may have been seen as engineering hurdles, but we believe these issues fall into the category of tolerance related research in optical and algorithmic designs.

## REFERENCES

- [1] Kaan Akşit, Ahmet Serdar Karadeniz, Praneeth Chakravarthula, Wang Yujie, Koray Kavaklı, Yuta Itoh, David Robert Walton, and Runze Zhu. 2022. *Odak*. <https://doi.org/10.5281/zenodo.6528486>
- [2] Ali Cem, M Kivanc Hedili, Erdem Ulusoy, and Hakan Urey. 2020. Foveated near-eye display using computational holography. *Scientific reports* 10, 1 (2020), 1–9.
- [3] Praneeth Chakravarthula, Zhan Zhang, Okan Tursun, Piotr Didyk, Qi Sun, and Henry Fuchs. 2021. Gaze-contingent retinal speckle suppression for perceptually-matched foveated holographic displays. *IEEE Transactions on Visualization and Computer Graphics* 27, 11 (2021), 4194–4203.
- [4] John C Heurtley. 1973. Scalar Rayleigh–Sommerfeld and Kirchhoff diffraction integrals: a comparison of exact evaluations for axial points. *JOSA* 63, 8 (1973), 1003–1008.
- [5] Koray Kavaklı, Hakan Urey, and Kaan Akşit. 2022. Learned holographic light transport: invited. *Appl. Opt.* 61, 5 (Feb 2022), B50–B55. <https://doi.org/10.1364/AO.439401>
- [6] George Alex Koulieris, Kaan Akşit, Michael Stengel, Rafał K Mantiuk, Katerina Mania, and Christian Richardt. 2019. Near-eye display and tracking technologies for virtual and augmented reality. In *Computer Graphics Forum*, Vol. 38. Wiley Online Library, 493–519.
- [7] Grace Kuo, Laura Waller, Ren Ng, and Andrew Maimone. 2020. High resolution étendue expansion for holographic displays. *ACM Transactions on Graphics (TOG)* 39, 4 (2020), 66–1.
- [8] Ghaith Makey, Özgün Yavuz, Denizhan K Kesim, Ahmet Turnalı, Parviz Elahi, Serim Ilday, Onur Tokel, and F Ömer Ilday. 2019. Breaking crosstalk limits to dynamic holography using orthogonality of high-dimensional random vectors. *Nature photonics* 13, 4 (2019), 251–256.
- [9] Liang Shi, Beichen Li, Changil Kim, Petr Kellnhofer, and Wojciech Matusik. 2021. Towards real-time photorealistic 3D holography with deep neural networks. *Nature* 591, 7849 (2021), 234–239.
- [10] Chris Slinger, Colin Cameron, and Maurice Stanley. 2005. Computer-generated holography as a generic display technology. *Computer* 38, 8 (2005), 46–53.
- [11] Maciej Sypek. 1995. Light propagation in the Fresnel region. New numerical approach. *Optics communications* 116, 1-3 (1995), 43–48.

- [12] David R. Walton, Koray Kavaklı, Rafael Kuffner Dos Anjos, David Swapp, Tim Weyrich, Hakan Urey, Anthony Steed, Tobias Ritschel, and Kaan Akşit. 2022. Metameric Varifocal Holograms. In *2022 IEEE Conference on Virtual Reality and 3D User Interfaces (VR)*. 746–755. <https://doi.org/10.1109/VR51125.2022.00096>

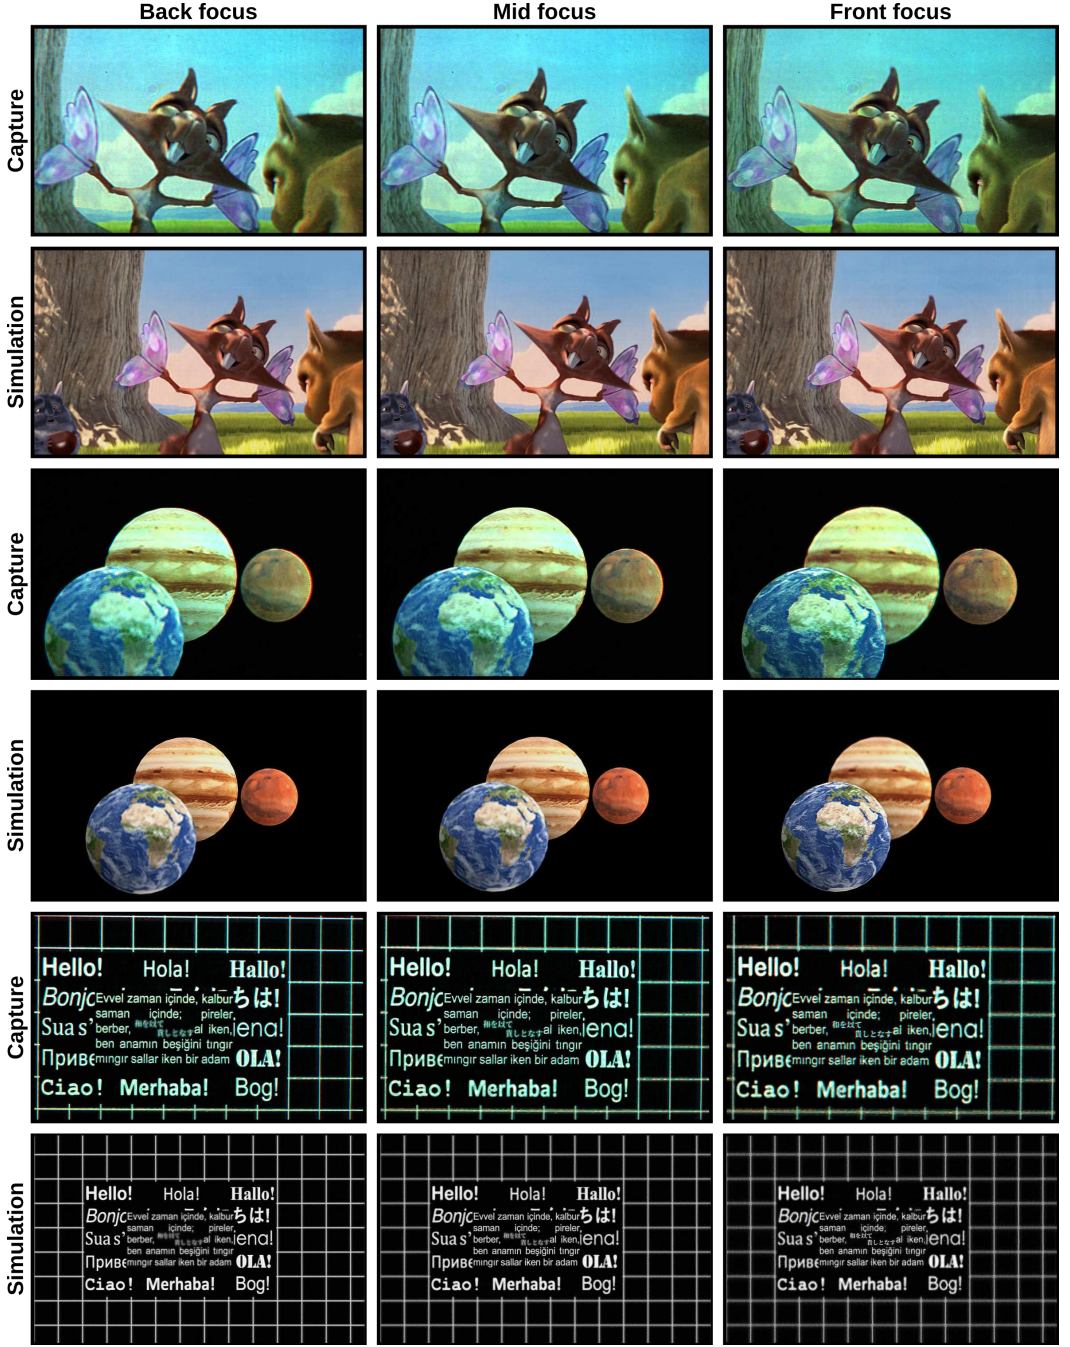

Fig. 2. Additional capture and simulation results of our method with various different scenes and focuses. The provided captures are generated on the Spatial Light Modulator (SLM) plane. All the images are captured with 20 ms exposure time using our holographic display. The provided simulated images are also generated on the Spatial Light Modulator (SLM) plane. All the simulated images are results from our hologram reconstruction simulation using our method. Both in captures and simulations, there are six target image planes in depth with 1 mm separation between each depth plane ( $-2.5$  mm and  $+2.5$  mm with respect to an SLM).

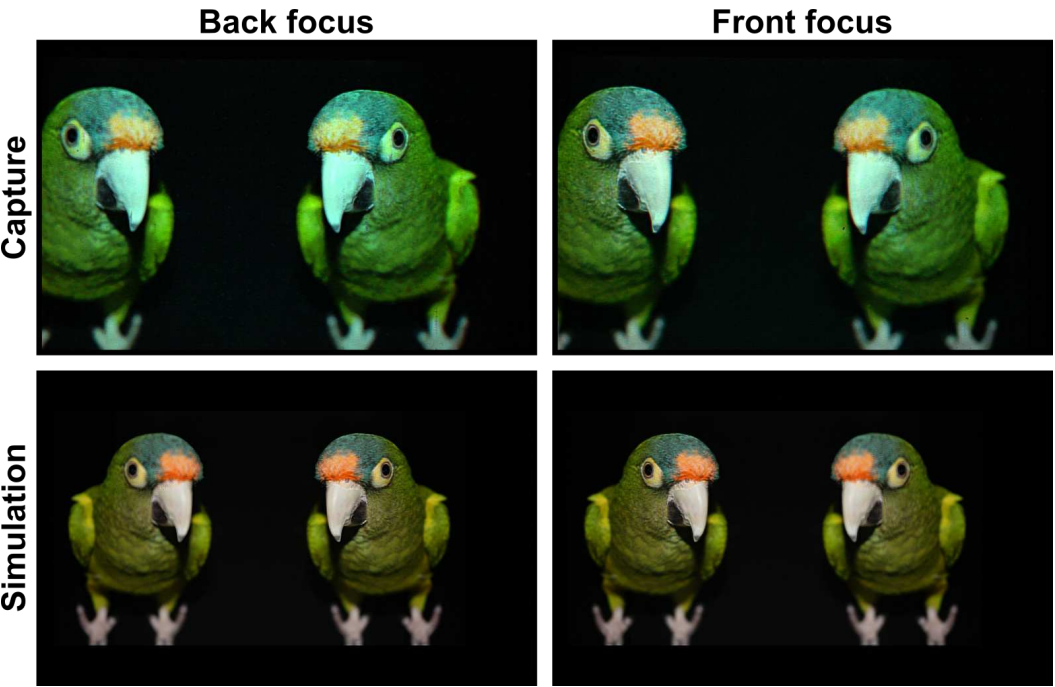

Fig. 3. Additional capture and simulation results of our method with various different scenes and focuses. The provided captures are generated on the Spatial Light Modulator (SLM) plane. All the images are captured with 20 ms exposure time using our holographic display. The provided simulated images are also generated on the Spatial Light Modulator (SLM) plane. All the simulated images are results from our hologram reconstruction simulation using our method. Both in captures and simulations, there are six target image planes in depth with 1 mm separation between each depth plane (-2.5 mm and +2.5 mm with respect to an SLM).

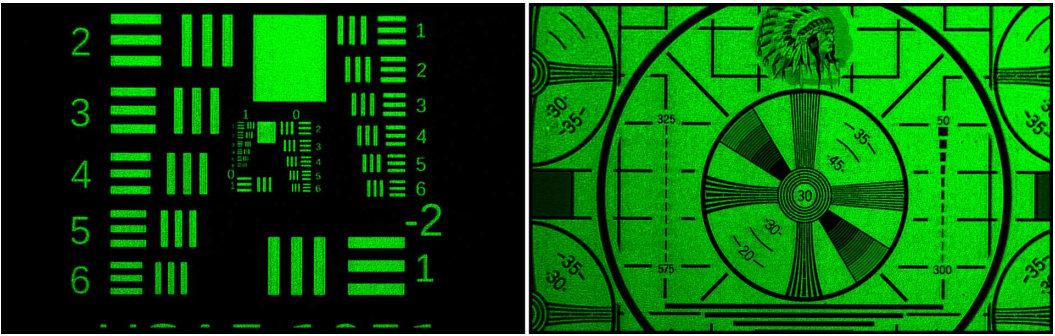

Fig. 4. Additional 2D captures. USAF 1951 and Indian Head Pattern charts demonstrate our holographic display prototype's resolution and contrast capability.

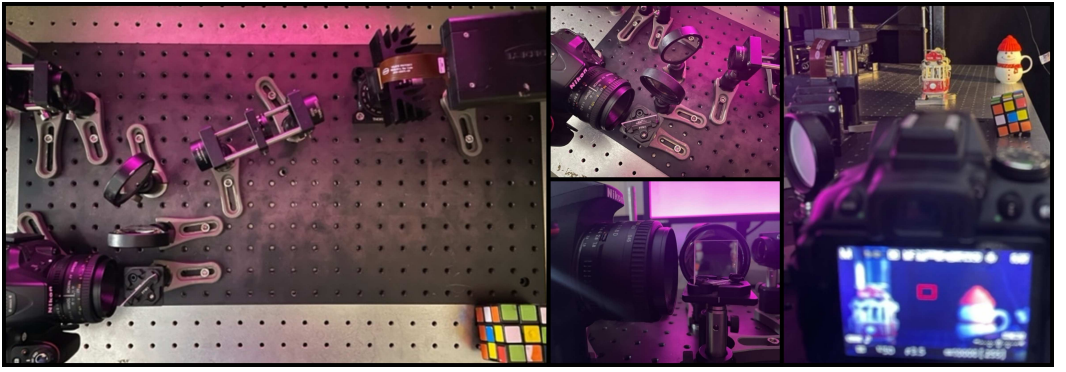

Fig. 5. Our proof-of-concept holographic display for Augmented Reality Near-Eye Display application example. Here, we provide various captures of our modified holographic display for AR near-eye display application. We additionally introduce a mirror, eyepiece lens and beam splitter to our display. The camera and the lens imitate the user's view with changing focus cues. The right image demonstrates the actual scene that we used in our captures. The Rubik's Cube, train, and snowman are located 45 cm, 65 cm, and 100 cm away from the camera.

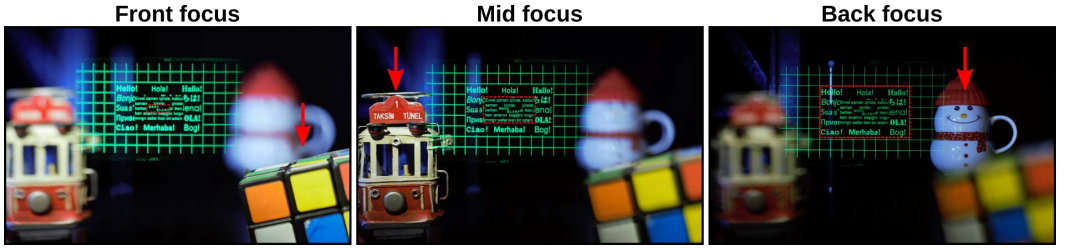

Fig. 6. Augmented Reality Near-Eye Display application example. Here, we provide samples from our modified holographic display approximating a baseline AR near-eye display. We show virtual images generated at various optical depths in the given scene. There are eight target image planes in depth with 1 mm separation between each depth plane (-3.5 mm and +3.5 mm with respect to an SLM). The focused virtual image planes correspond to 45 cm, 65 cm, and 100 cm with respect to the user's view. We indicate these plane locations with real objects (Rubik's Cube, train, and snowman) that are placed on the target distances. The red boxes and arrows indicate the focused depth plane in the captures.

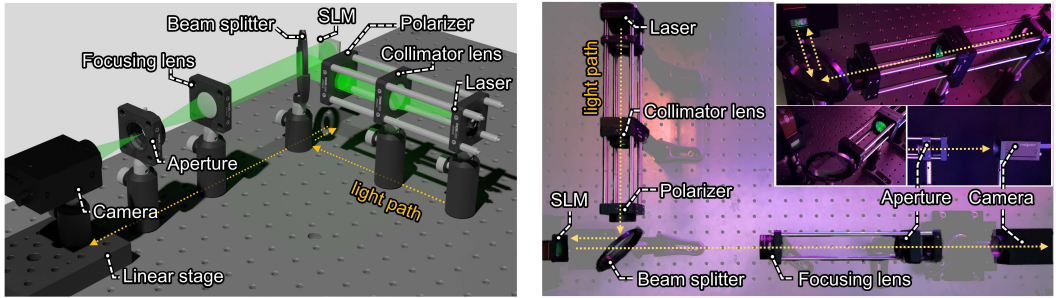

Fig. 7. Our proof-of-concept holographic display for long projection distances. (Left) A three-dimensional layout of our design shows the arrangement of our prototype’s optical and optomechanical components. (Right) A photograph of our proof-of-concept holographic display setup with annotations of primary components. Both at the layout and photographs, light direction and path are indicated with a yellow line.

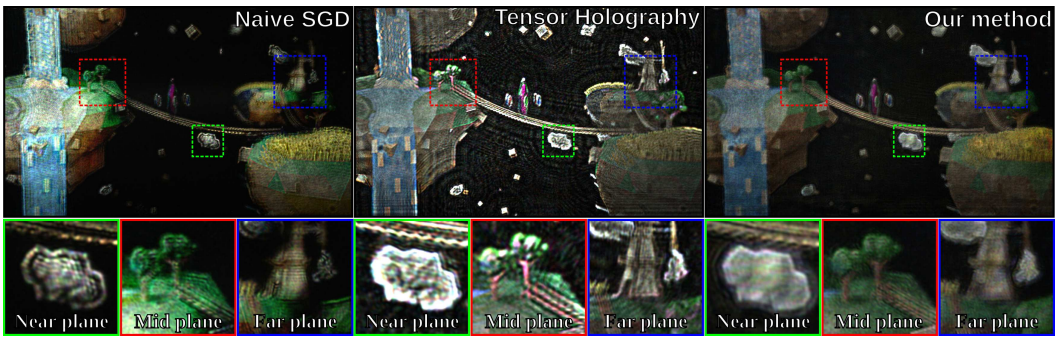

Fig. 8. Support for long projection distances. Here, we provide captures from our holographic display at a projection distance of 15 cm. The indicated focuses of near, mid and far correspond to 14.0 cm, 14.5 cm and 15.0 cm, respectively. Our method maintains image quality at these projection distances, unlike the literature’s state of the art methods.
